# Supplementary material for: Gas Sensing Properties of Novel Indium Oxide Monolayer: A First-Principles Study
Source: arXiv:2509.05121 source file (2025-09-05)
Supplement: Supplementary file 1 [file Supplementary.pdf]

# Gas Sensing Properties of Novel Indium Oxide monolayer: A First-Principles Study

Afreen Anamul Haque, Suraj G. Dhongade, and Aniket Singha\*

*Department of Electronics and Electrical Communication Engineering, Indian Institute of  
Technology Kharagpur, Kharagpur-721302, India*

E-mail: [aniket@ece.iitkgp.ac.in](mailto:aniket@ece.iitkgp.ac.in)

### A1. Methodology for Initial Adsorption Site Selection and Structural Optimization

The adsorption of gas molecules on a monolayer surface preferentially occurs at the site with the most negative adsorption energy, corresponding to the most thermodynamically stable configuration of the gas–monolayer system. To identify such a configuration, the system was subjected to structural relaxation by initially placing the gas molecule at various high-symmetry sites on the monolayer surface. These initial adsorption sites were systematically selected based on symmetry considerations, as illustrated in Fig. S1: (i) atop a top-layer Indium (In) atom, (ii) atop a top-layer Oxygen (O) atom, (iii) above a middle-layer Oxygen atom (hollow site), (iv) at the midpoint of the bond between a top-layer In and O atom, and (v) at the midpoint of the bridge between two top-layer In atoms. Gas molecules were placed in both vertical and horizontal orientations at each of these six adsorption sites. For polar molecules such as ammonia ( $\text{NH}_3$ ) and water ( $\text{H}_2\text{O}$ ), the effect of molecular dipole orientation was explored by aligning different molecular ends towards the surface. An initial vertical separation of 2.5 Å was maintained between each molecule and the surface. Structural relaxation was subsequently performed for all initial configurations, and the most energetically favorable structure was determined to represent the most stable adsorption configuration for each gas species. Due to the symmetry of the hexagonal lattice, certain geometries converged to equivalent energy minima. This comprehensive methodology enabled the determination of the most favorable adsorption sites and configurations based on minimum energy criteria. Representative top and side views of the lowest-energy configurations for all ten harmful gas molecules and three ambient molecules under consideration are presented in Figure S1.

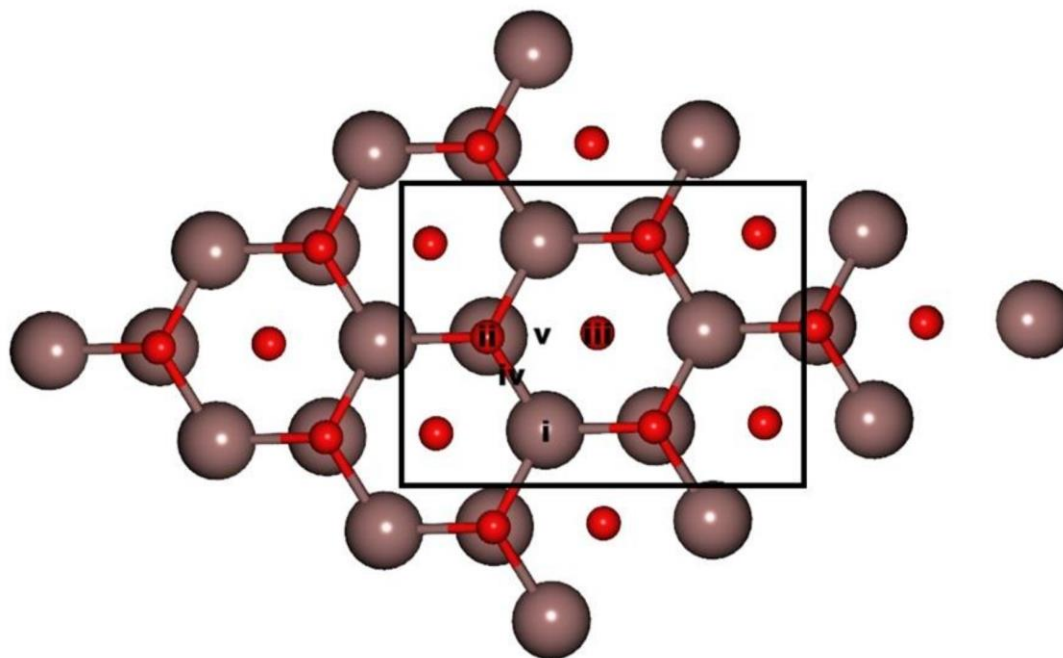

Fig. S1: Top view of a  $3 \times 3 \times 1$   $\text{In}_2\text{O}_3$  monolayer supercell, highlighting the identified initial adsorption sites (high symmetry sites): (i) atop a top-layer Indium (In) atom, (ii) atop a top-layer Oxygen (O) atom, (iii) above a middle-layer Oxygen atom (hollow site), (iv) at the midpoint of the bond between a top-layer In and O atom, and (v) at the midpoint of the bridge between two top-layer In atoms. Atom color coding: Indium (In) – greyish brown; Oxygen (O) – red.

**A2. Top and side views of the monolayer with adsorbed molecules in the most stable configuration**

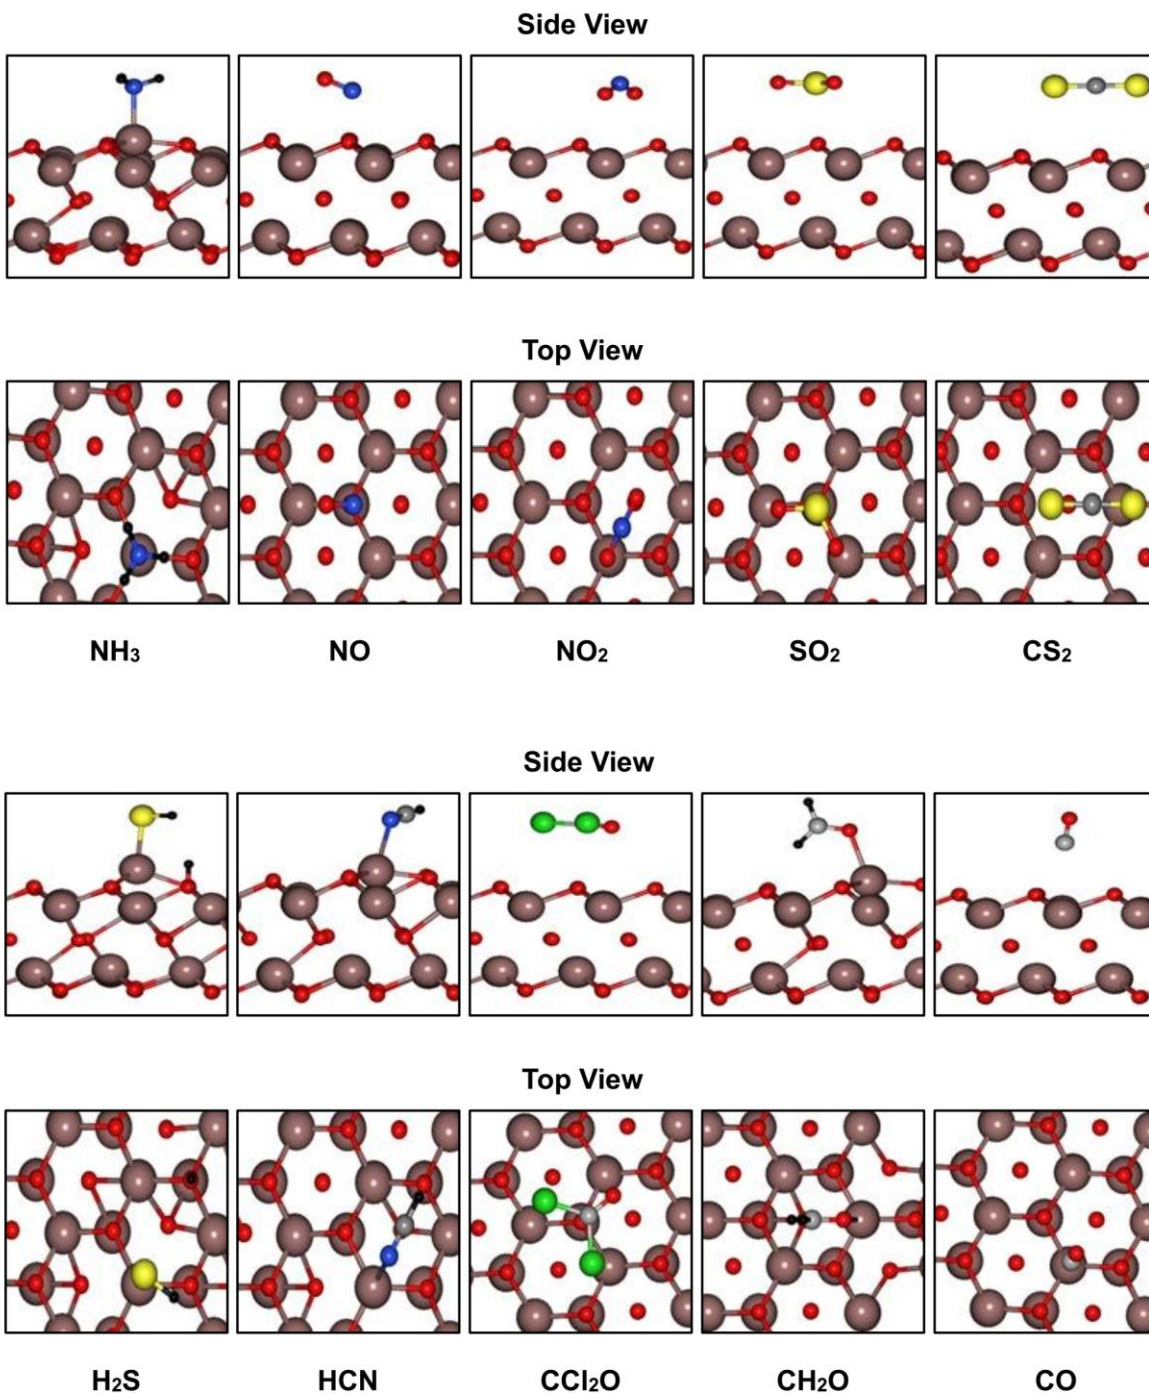

Fig. S2: Top and side views of the most stable adsorption configurations of the  $\text{In}_2\text{O}_3$  monolayer for the ten toxic gas molecules under investigation. Atoms are color-coded as follows: Indium (In) – greyish brown, Oxygen (O) – red, Nitrogen (N) – blue, Hydrogen (H) – black, Carbon (C) – grey, Sulfur (S) – yellow, and Chlorine (Cl) – green.

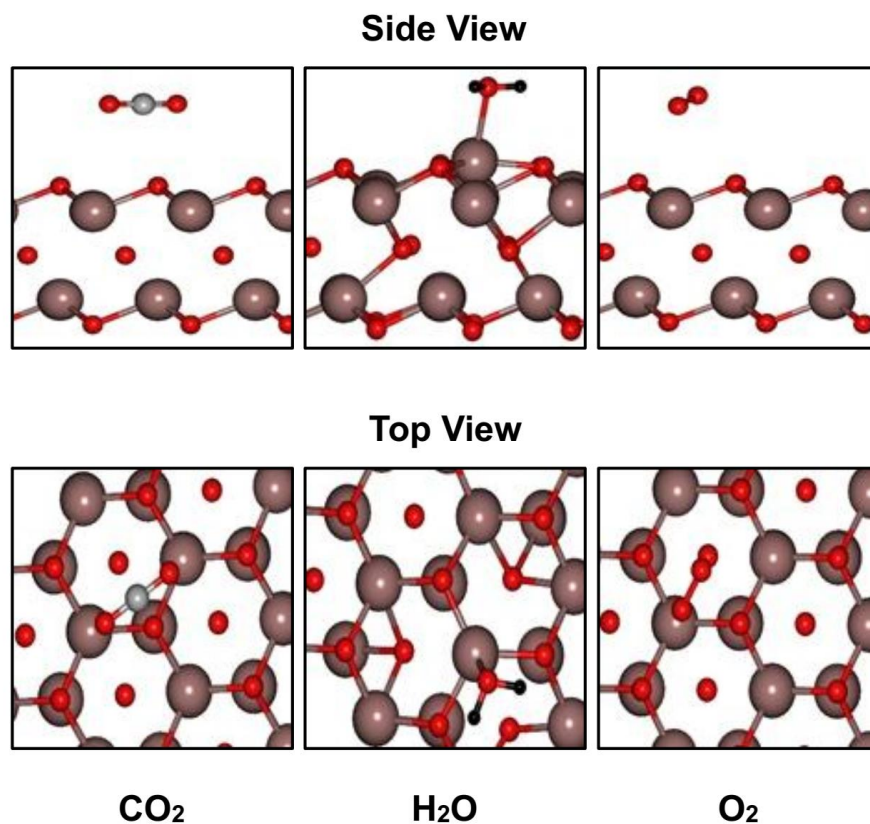

Fig. S3: Top and side views of the most stable adsorption configurations of the  $\text{In}_2\text{O}_3$  monolayer for the three atmospheric gas molecules under study. Atoms are color-coded as follows: Indium (In) – greyish brown, Oxygen (O) – red, Hydrogen (H) – black, and Carbon (C) – grey.

### A3: Comparison of gas adsorption energy and recovery time from literature with In<sub>2</sub>O<sub>3</sub> monolayer for NH<sub>3</sub>, NO, H<sub>2</sub>S, HCN, CH<sub>2</sub>O and H<sub>2</sub>O molecules which demonstrate E<sub>ads</sub><-0.4eV

TABLE I

THEORETICAL STUDY OF THE NH<sub>3</sub> ADSORPTION ON DIFFERENT 2D MATERIALS FROM THE LITERATURE, HIGHLIGHTING ADSORPTION ENERGY AND RECOVERY TIME BASED ON DFT CALCULATIONS.

| System                                                | E <sub>ads</sub> (eV) | τ (s)                    | Functional |
|-------------------------------------------------------|-----------------------|--------------------------|------------|
| In <sub>2</sub> Se <sub>3</sub> (bottom) [1]          | -0.49                 | 1.70 x 10 <sup>-4</sup>  | GGA-PBE    |
| In <sub>2</sub> Se <sub>3</sub> (top) [1]             | -0.19                 | 1.56 x 10 <sup>-9</sup>  | GGA-PBE    |
| MoS <sub>2</sub> [2]                                  | -0.02                 | 2.53 x 10 <sup>-12</sup> | GGA-PBE    |
| Cu-doped WS <sub>2</sub> [3]                          | -1.02                 | 1.85 x 10 <sup>5</sup>   | GGA-PBE    |
| WS <sub>2</sub> [4]                                   | 0.31                  | 5.96 x 10 <sup>-18</sup> | GGA-PBE    |
| Graphene [5]                                          | -0.11                 | 7.05 x 10 <sup>-11</sup> | LDA        |
| B-doped Graphene [5]                                  | -0.50                 | 2.51 x 10 <sup>-4</sup>  | LDA        |
| Phosphorene [6]                                       | -0.18                 | 1.06 x 10 <sup>-9</sup>  | optB88     |
| Silicene [7]                                          | -0.60                 | 1.20 x 10 <sup>-2</sup>  | GGA-PBE    |
| Hexagonal Ga <sub>2</sub> O <sub>3</sub> (top) [8]    | -1.19                 | 1.06 x 10 <sup>8</sup>   | GGA-PBE    |
| Hexagonal Ga <sub>2</sub> O <sub>3</sub> (bottom) [8] | -0.41                 | 7.72 x 10 <sup>-6</sup>  | GGA-PBE    |
| Ga <sub>2</sub> O <sub>2</sub> [9]                    | -0.54                 | 1.45 x 10 <sup>-3</sup>  | GGA-PBE    |
| In <sub>2</sub> O <sub>3</sub> (this work)            | -1.07                 | 8.17 x 10 <sup>5</sup>   | GGA-PBE    |

TABLE II

THEORETICAL STUDY OF THE NO ADSORPTION ON DIFFERENT 2D MATERIALS FROM THE LITERATURE, HIGHLIGHTING ADSORPTION ENERGY AND RECOVERY TIME BASED ON DFT CALCULATIONS.

| System                                                | E <sub>ads</sub> (eV) | τ (ms)                  | Functional |
|-------------------------------------------------------|-----------------------|-------------------------|------------|
| In <sub>2</sub> Se <sub>3</sub> (bottom) [1]          | -0.19                 | 1.63 x 10 <sup>-6</sup> | GGA-PBE    |
| In <sub>2</sub> Se <sub>3</sub> (top) [1]             | -0.12                 | 9.89 x 10 <sup>-8</sup> | GGA-PBE    |
| MoS <sub>2</sub> [2]                                  | -0.03                 | 3.61 x 10 <sup>-9</sup> | GGA-PBE    |
| WS <sub>2</sub> [4]                                   | -0.25                 | 1.58 x 10 <sup>-7</sup> | GGA-PBE    |
| Graphene [5]                                          | -0.30                 | 1.18 x 10 <sup>-4</sup> | LDA        |
| B-doped Graphene [5]                                  | -1.07                 | 1.25 x 10 <sup>3</sup>  | LDA        |
| Phosphorene [6]                                       | -0.32                 | 2.58 x 10 <sup>-4</sup> | optB88     |
| Silicene [7]                                          | -0.57                 | 4.36                    | GGA-PBE    |
| Hexagonal Ga <sub>2</sub> O <sub>3</sub> (top) [8]    | -0.60                 | 19.2                    | GGA-PBE    |
| Hexagonal Ga <sub>2</sub> O <sub>3</sub> (bottom) [8] | -0.15                 | 3.31 x 10 <sup>-7</sup> | GGA-PBE    |
| Ga <sub>2</sub> O <sub>2</sub>                        | -0.26                 | 2.76 x 10 <sup>-5</sup> | GGA-PBE    |
| In <sub>2</sub> O <sub>3</sub> (this work)            | -0.68                 | 197                     | GGA-PBE    |

TABLE III

THEORETICAL STUDY OF THE H<sub>2</sub>S ADSORPTION ON DIFFERENT 2D MATERIALS FROM THE LITERATURE, HIGHLIGHTING ADSORPTION ENERGY AND RECOVERY TIME BASED ON DFT CALCULATIONS.

| System                                                 | E <sub>ads</sub> (eV) | τ (s)                           | Functional |
|--------------------------------------------------------|-----------------------|---------------------------------|------------|
| Penta PdAs <sub>2</sub> (bottom) [10]                  | -0.49                 | 1.79 x 10 <sup>-6</sup>         | GGA-PBE    |
| MoWC based MXenes (Mo side) [11]                       | -1.15                 | 2.213 x 10 <sup>7</sup> (300K)  | GGA-PBE    |
| MoWC based MXenes (W side) [11]                        | -0.95                 | 1.311 x 10 <sup>4</sup> (300K)  | GGA-PBE    |
| MoWCO <sub>2</sub> based MXenes (Mo side) [11]         | -0.29                 | 8.543 x 10 <sup>-8</sup> (300K) | GGA-PBE    |
| MoWCO <sub>2</sub> based MXenes (W side) [11]          | -0.32                 | 5.222 x 10 <sup>-9</sup> (300K) | GGA-PBE    |
| GeC [12]                                               | -0.20                 | 3.04 x 10 <sup>-9</sup>         | GGA-PBE    |
| CoOOH [13]                                             | -0.43                 | -                               | GGA-PBE    |
| Hexagonal Ga <sub>2</sub> O <sub>3</sub> (top) [14]    | -0.19                 | -                               | GGA-PBE    |
| Hexagonal Ga <sub>2</sub> O <sub>3</sub> (bottom) [14] | -0.31                 | -                               | GGA-PBE    |
| Graphene [15]                                          | -0.61                 | -                               | GGA-PBE    |
| Au-doped Graphene [15]                                 | -0.90                 | -                               | GGA-PBE    |
| Bilayer Graphene [16]                                  | -0.16                 | -                               | GGA-PBE    |
| Pristine MoSe <sub>2</sub> [17]                        | -0.35                 | 7.59 x 10 <sup>-7</sup> (300K)  | GGA-PBE    |
| Ru-doped MoSe <sub>2</sub> [17]                        | -1.13                 | 9.63 x 10 <sup>6</sup> (300K)   | GGA-PBE    |
| Rh-doped MoSe <sub>2</sub> [17]                        | -1.04                 | 2.96 x 10 <sup>5</sup> (300K)   | GGA-PBE    |
| Pd-doped MoSe <sub>2</sub> [17]                        | -1.02                 | 1.36 x 10 <sup>5</sup> (300K)   | GGA-PBE    |
| MoO <sub>3</sub> [18]                                  | -0.5                  | -                               | GGA-PBE    |
| In <sub>2</sub> O <sub>3</sub> (this work)             | -1.29                 | 3.63 x 10 <sup>9</sup>          | GGA-PBE    |



TABLE IV

THEORETICAL STUDY OF THE HCN ADSORPTION ON DIFFERENT 2D MATERIALS FROM THE LITERATURE, HIGHLIGHTING ADSORPTION ENERGY AND RECOVERY TIME BASED ON DFT CALCULATIONS.

| System                                            | $E_{\text{ads}}$ (eV) | $\tau$ (s)                   | Functional |
|---------------------------------------------------|-----------------------|------------------------------|------------|
| Pristine MoSe <sub>2</sub> [17]                   | -0.27                 | $3.44 \times 10^{-8}$ (300K) | GGA-PBE    |
| Ru-doped MoSe <sub>2</sub> [17]                   | -1.71                 | 6.39 (673K)                  | GGA-PBE    |
| Rh-doped MoSe <sub>2</sub> [17]                   | -0.85                 | 18.32(323K)                  | GGA-PBE    |
| Pd-doped MoSe <sub>2</sub> [17]                   | -0.78                 | 12.70 (300K)                 | GGA-PBE    |
| Ta-doped MoSe <sub>2</sub> (W side) [19]          | -0.98                 | 4.64 (390K)                  | GGA-PBE    |
| B <sub>6</sub> N <sub>6</sub> H <sub>6</sub> [20] | -0.31                 | $1.00 \times 10^{-6}$ (300K) | GGA-PBE    |
| CoOOH [13]                                        | -0.80                 | 339 (298K)                   | GGA-PBE    |
| Al-doped Graphene [21]                            | -1.67                 | -                            | X3LYP      |
| Si-doped Graphene [21]                            | -1.17                 | -                            | X3LYP      |
| Phosphorene [22]                                  | -0.24                 | -                            | GGA-PBE    |
| Al-doped Phosphorene [22]                         | -0.59                 | -                            | GGA-PBE    |
| Si-doped Phosphorene [22]                         | -0.19                 | -                            | GGA-PBE    |
| S-doped Phosphorene [22]                          | -0.19                 | -                            | GGA-PBE    |
| In <sub>2</sub> O <sub>3</sub> (this work)        | -0.46                 | $5.43 \times 10^{-5}$        | GGA-PBE    |

TABLE V

THEORETICAL STUDY OF THE CH<sub>2</sub>O ADSORPTION ON DIFFERENT 2D MATERIALS FROM THE LITERATURE, HIGHLIGHTING ADSORPTION ENERGY AND RECOVERY TIME BASED ON DFT CALCULATIONS.

| System                                        | $E_{\text{ads}}$ (eV) | $\tau$ (s)             | Functional |
|-----------------------------------------------|-----------------------|------------------------|------------|
| BN [23]                                       | -0.28                 | $5.06 \times 10^{-8}$  | GGA-PBE    |
| AlN [23]                                      | -1.04                 | $2.96 \times 10^5$     | GGA-PBE    |
| GaN [23]                                      | -0.46                 | $5.34 \times 10^{-5}$  | GGA-PBE    |
| InN [23]                                      | -1.05                 | $4.36 \times 10^5$     | GGA-PBE    |
| BP [23]                                       | -0.25                 | $1.58 \times 10^{-8}$  | GGA-PBE    |
| P [23]                                        | -0.19                 | $1.56 \times 10^{-9}$  | GGA-PBE    |
| GeC [24]                                      | -0.27                 | $8.76 \times 10^{-10}$ | GGA-PBE    |
| 2D B <sub>3</sub> O <sub>3</sub> [25]         | -0.35                 | $8.1 \times 10^{-7}$   | GGA-PBE    |
| 2D Ga <sub>2</sub> O <sub>2</sub> [9]         | -0.64                 | $5.64 \times 10^{-2}$  | GGA-PBE    |
| 2D In <sub>2</sub> O <sub>3</sub> (this work) | -0.64                 | $5.64 \times 10^{-2}$  | GGA-PBE    |

TABLE VI

THEORETICAL STUDY OF THE H<sub>2</sub>O ADSORPTION ON DIFFERENT 2D MATERIALS FROM THE LITERATURE, HIGHLIGHTING ADSORPTION ENERGY AND RECOVERY TIME BASED ON DFT CALCULATIONS.

| System                                                  | $E_{\text{ads}}$ (eV) | $\tau$ (s)             | Functional   |
|---------------------------------------------------------|-----------------------|------------------------|--------------|
| Monolayer MoS <sub>2</sub> edges [26]                   | -0.55                 | $1.74 \times 10^{-3}$  | GGA-PBE      |
| 2D Ferromagnetic Fe <sub>3</sub> GeTe <sub>2</sub> [27] | -0.25                 | $1.85 \times 10^{-8}$  | GGA-PBE      |
| defective-Fe <sub>3</sub> GeTe <sub>2</sub> [27]        | -0.76                 | 5.85                   | GGA-PBE      |
| Monolayer Pt(111) [28]                                  | -0.42                 | $1.14 \times 10^{-5}$  | vdW-DF2-B86R |
| GeC [24]                                                | -0.27                 | $8.76 \times 10^{-10}$ | GGA-PBE      |
| 2D Ga <sub>2</sub> O <sub>2</sub> [9]                   | -0.19                 | $1.94 \times 10^{-9}$  | GGA-PBE      |
| 2D In <sub>2</sub> O <sub>3</sub> (this work)           | -0.63                 | $3.83 \times 10^{-2}$  | GGA-PBE      |

#### A4. DOS Profiles of Gas-Adsorbed In<sub>2</sub>O<sub>3</sub> Monolayer Systems Under 3% Tensile Strain

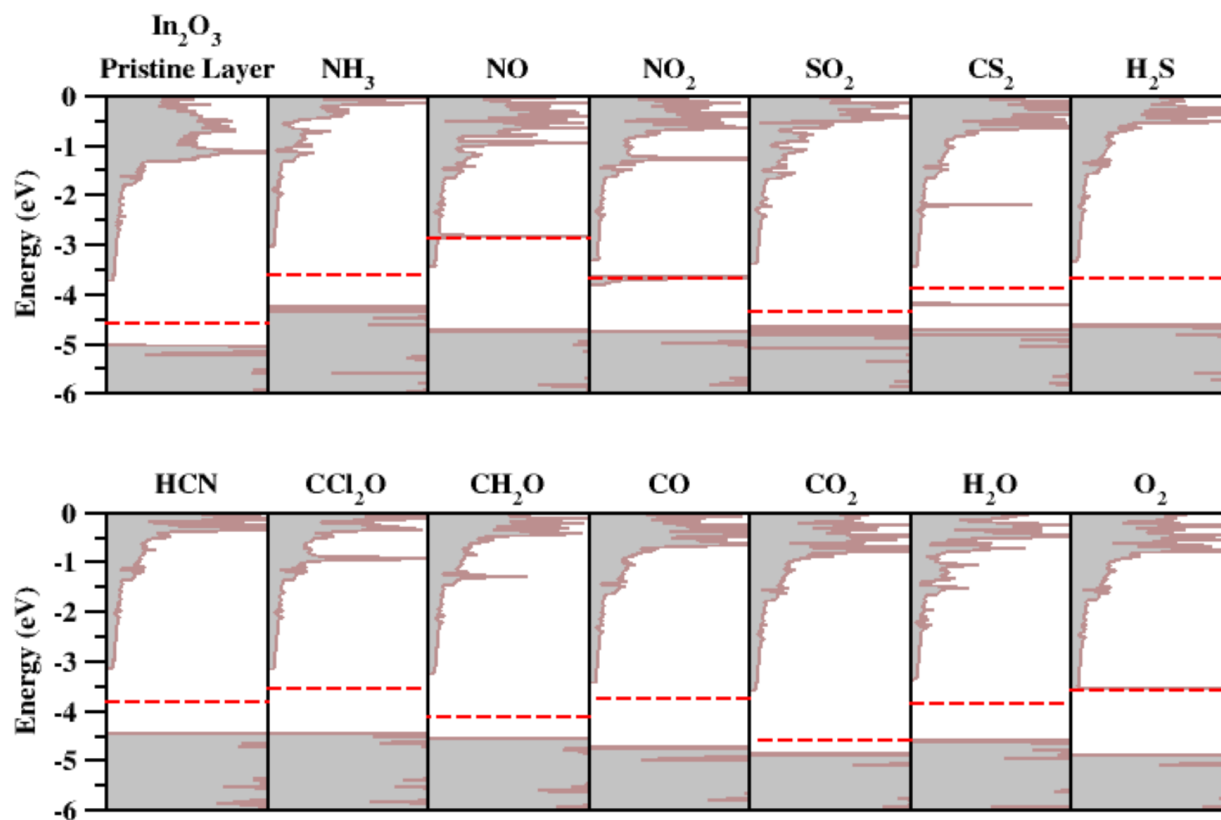

Fig. S4: Total density of states (TDOS) profiles for the molecule–monolayer systems under investigation, with 3% tensile strain applied to the In<sub>2</sub>O<sub>3</sub> monolayer. In all cases, the intrinsic Fermi level is indicated by a red dashed line.

## A5. DOS Profiles of Gas-Adsorbed $\text{In}_2\text{O}_3$ Monolayer Systems Under 2% Compressive Strain

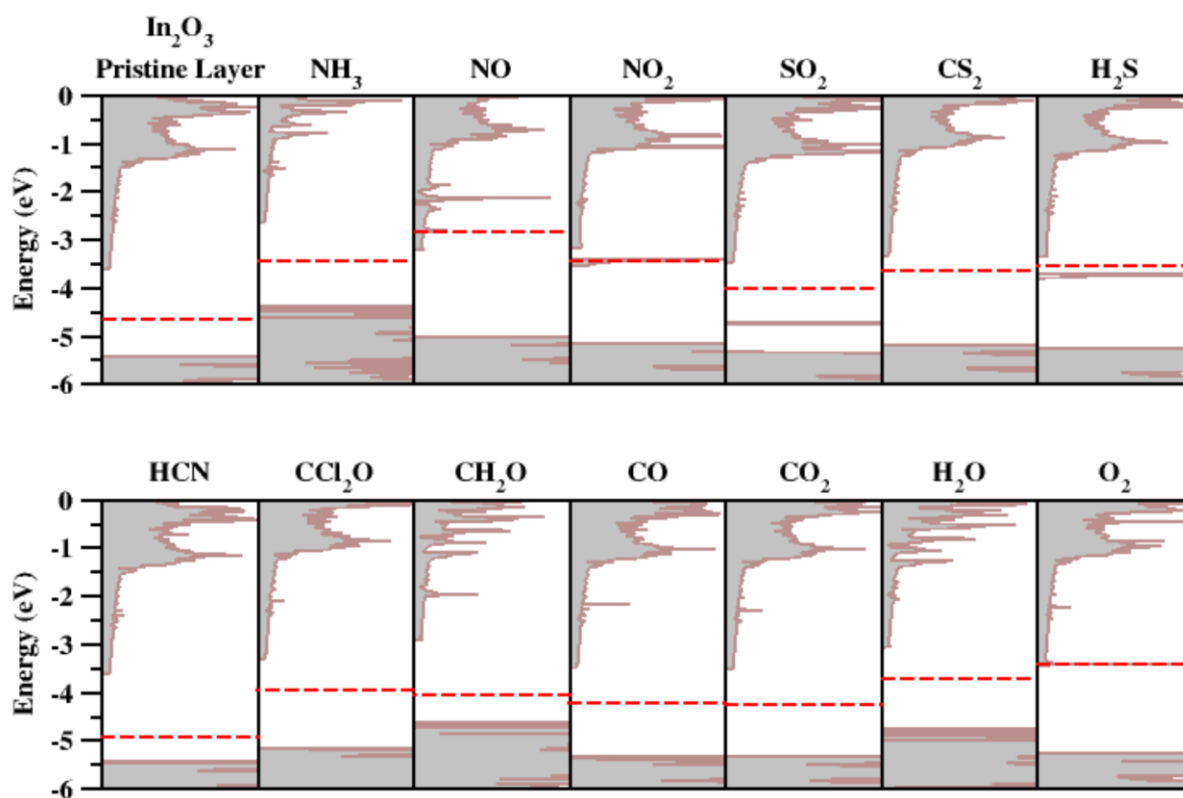

Fig. S5: Total density of states (TDOS) profiles for the molecule–monolayer systems under investigation, with 2% compressive strain applied to the  $\text{In}_2\text{O}_3$  monolayer. In all cases, the intrinsic Fermi level is indicated by a red dashed line.



## A6. Average Potential Profiles of 2D In<sub>2</sub>O<sub>3</sub> Monolayer–Gas Molecule Configurations Without Applied Strain

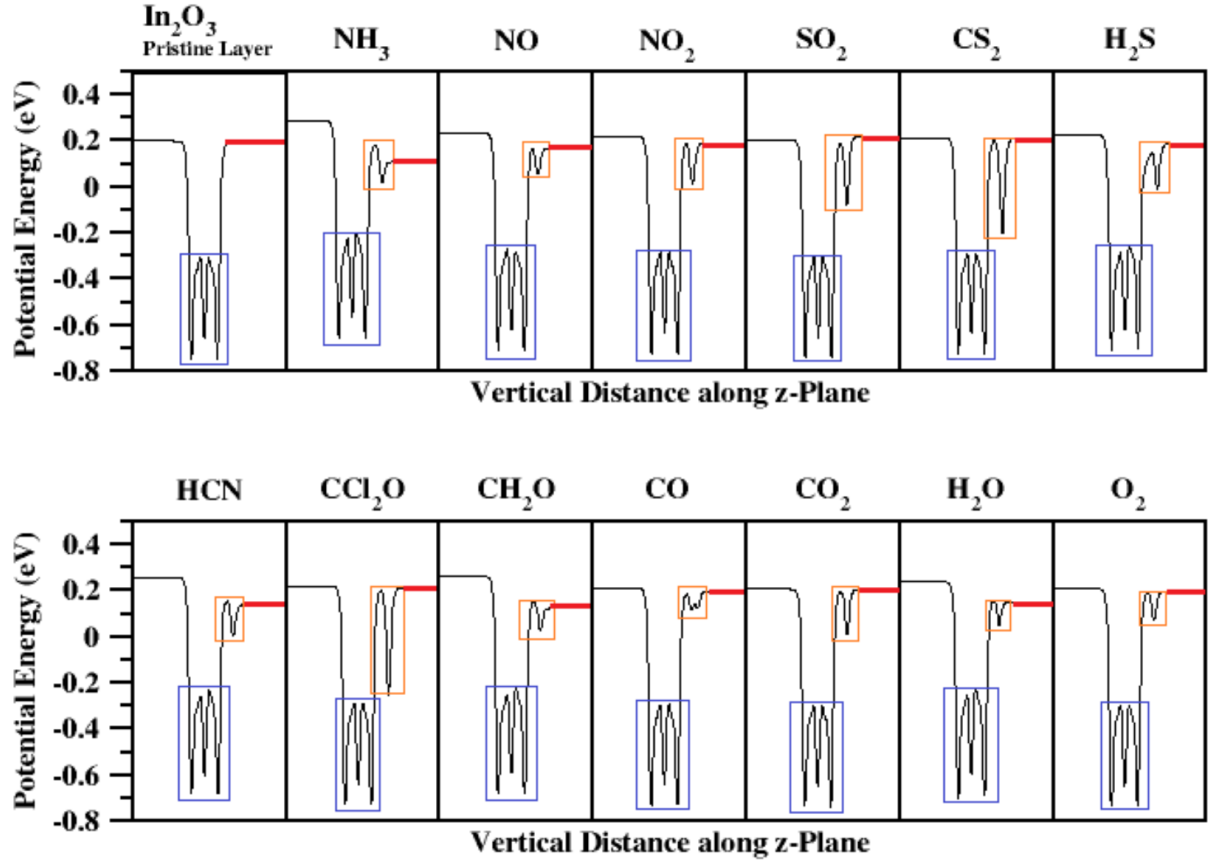

Fig. S6: Average electrostatic potential profile for the pristine In<sub>2</sub>O<sub>3</sub> monolayer and the gas-adsorbed configurations of the monolayer without applied strain. The blue-shaded region corresponds to the potential variation due to the atoms of the 2D monolayer, while the amber-shaded region represents the effect of the adsorbed gas molecule on the potential profile. The potential is plotted along the axis perpendicular to the monolayer plane (x-axis). The red horizontal line denotes the vacuum potential of the surface with the adsorbed gas molecule, and is used as  $E_{vac}$  in Eqn (6) for the calculation of the work function in the main paper.

$$\phi = E_{vac} - E_f$$

## A7. Average Potential Profiles of 2D In<sub>2</sub>O<sub>3</sub> Monolayer–Gas Molecule Configurations Under 3% Tensile Strain

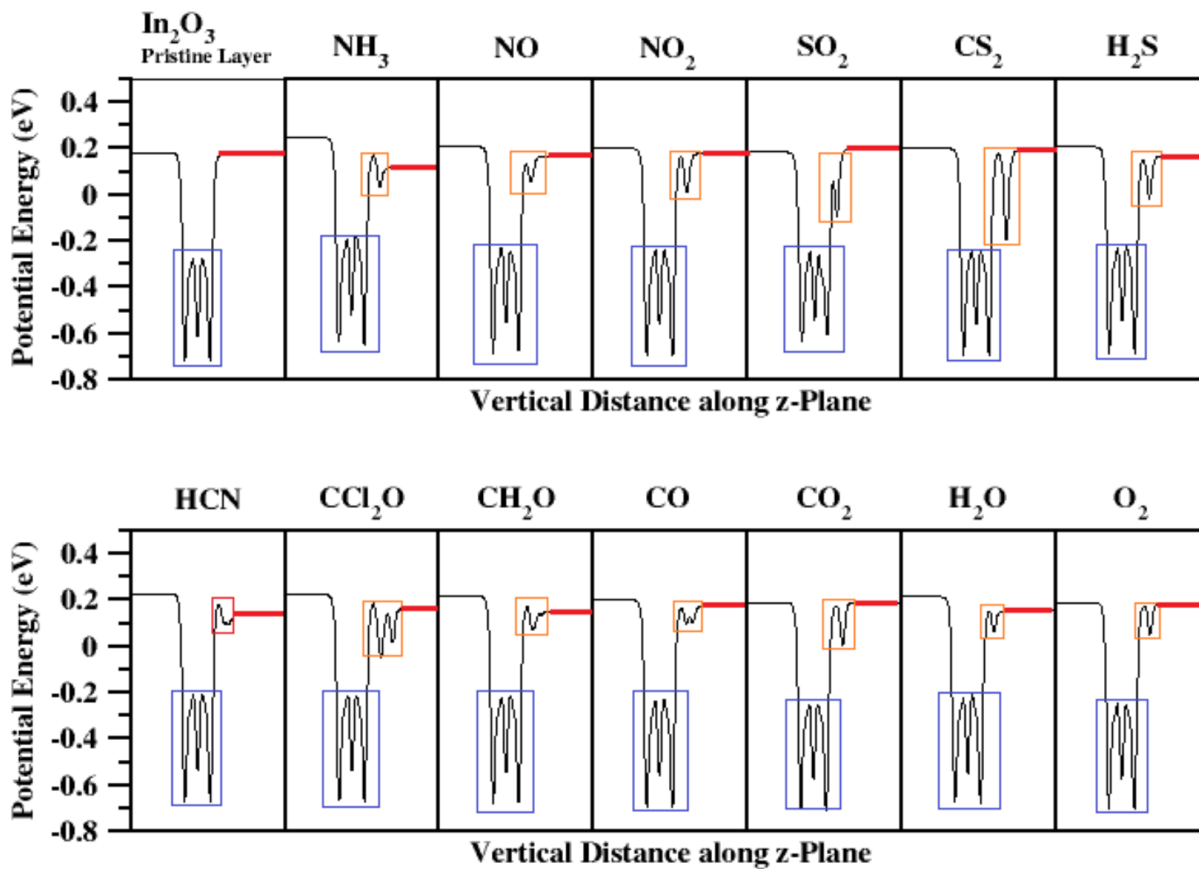

Fig. S7: Average electrostatic potential profile for the pristine In<sub>2</sub>O<sub>3</sub> monolayer and the gas-adsorbed configurations of the monolayer with 3% tensile strain. The blue-shaded region corresponds to the potential variation due to the atoms of the 2D monolayer, while the amber-shaded region represents the effect of the adsorbed gas molecule on the potential profile. The potential is plotted along the axis perpendicular to the monolayer plane (x-axis). The red horizontal line denotes the vacuum potential of the surface with the adsorbed gas molecule, and is used as  $E_{vac}$  in Eqn (6) for the calculation of the work function in the main paper:  $\phi = E_{vac} - E_f$

## A8. Average Potential Profiles of 2D In<sub>2</sub>O<sub>3</sub> Monolayer–Gas Molecule Configurations Under 2% Compressive Strain

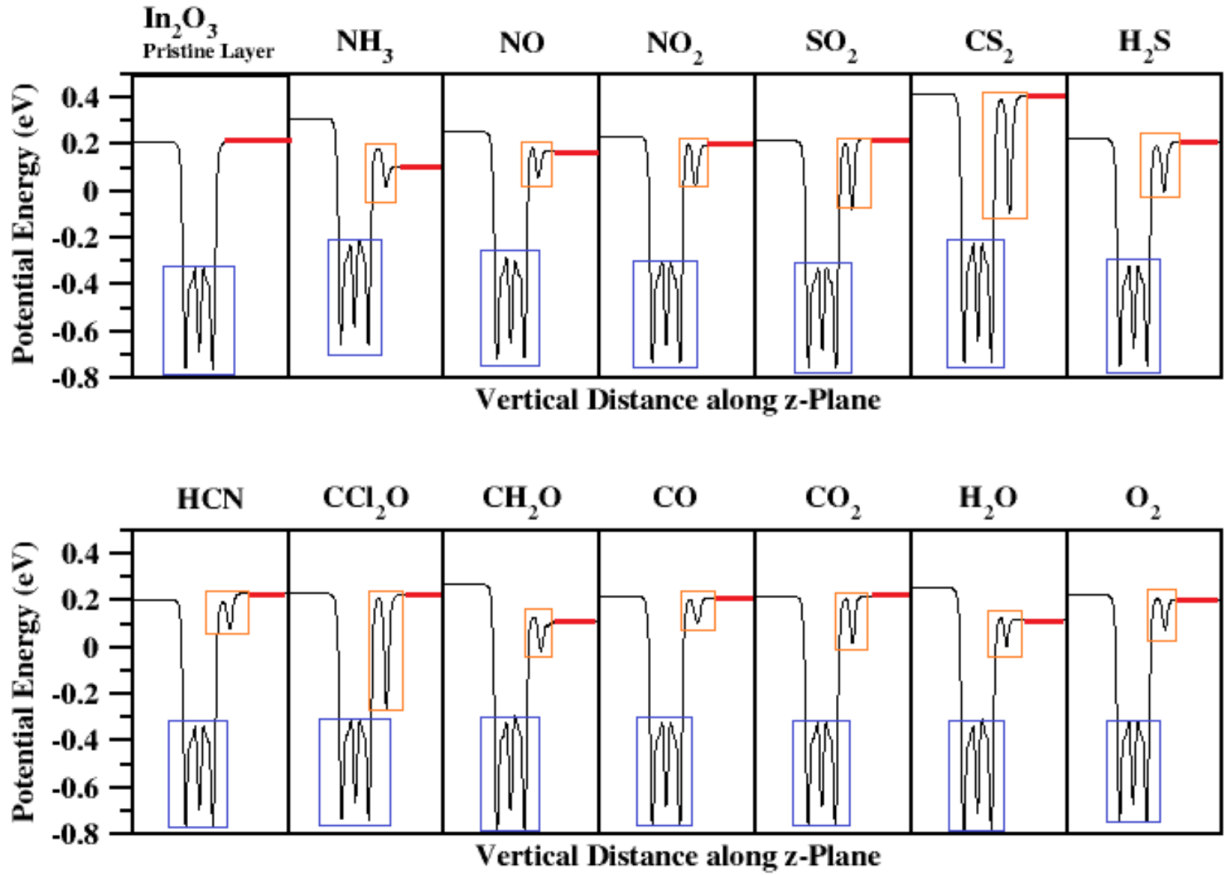

Fig. S8: Average electrostatic potential profile for the pristine In<sub>2</sub>O<sub>3</sub> monolayer and the gas-adsorbed configurations of the monolayer with 2% compressive strain. The blue-shaded region corresponds to the potential variation due to the atoms of the 2D monolayer, while the amber-shaded region represents the effect of the adsorbed gas molecule on the potential profile. The potential is plotted along the axis perpendicular to the monolayer plane (x-axis). The red horizontal line denotes the vacuum potential of the surface with the adsorbed gas molecule, and is used as  $E_{vac}$  in Eqn (6) for the calculation of the work function in the main paper:  $\phi = E_{vac} - E_f$

## REFERENCES

- [1] Q. Yue, Z. Shao, S. Chang, and J. Li, "Adsorption of gas molecules on monolayer mos2 and effect of applied electric field," *Nanoscale research letters*, vol. 8, no. 1, pp. 1–7, 2013.
- [2] D. Zhao, Y. Wen, Z. Li, Y. Cui, Y. Zhao, T.-F. Lu, M. He, B. Song, and Z. Zhang, "Theoretical study of adsorption of gas (co, co2, nh3) by metal (au, ag, cu)-doped single-layer ws2," *Journal of Molecular Modeling*, vol. 30, no. 10, p. 322, 2024.
- [3] V. Q. Bui, T.-T. Pham, D. A. Le, C. M. Thi, and H. M. Le, "A first-principles investigation of various gas (co, h2o, no, and o2) absorptions on a ws2 monolayer: stability and electronic properties," *Journal of Physics: Condensed Matter*, vol. 27, no. 30, p. 305005, 2015.
- [4] Z. Yonghui, C. Yabin, Z. Kaige, L. Caihong, Z. Jing, Z. Haoli, E. Peng Yong *et al.*, "Improving gas sensing properties of graphene by introducing dopants and defects: a first-principles study," *Nanotechnology (Print)*, vol. 20, 2009.
- [5] Y. Cai, Q. Ke, G. Zhang, and Y.-W. Zhang, "Energetics, charge transfer, and magnetism of small molecules physisorbed on phosphorene," *The Journal of Physical Chemistry C*, vol. 119, no. 6, pp. 3102–3110, 2015.
- [6] W. Hu, N. Xia, X. Wu, Z. Li, and J. Yang, "Silicene as a highly sensitive molecule sensor for nh 3, no and no 2," *Physical Chemistry Chemical Physics*, vol. 16, no. 15, pp. 6957–6962, 2014.
- [7] J. Zhao, X. Huang, Y. Yin, Y. Liao, H. Mo, Q. Qian, Y. Guo, X. Chen, Z. Zhang, and M. Hua, "Two-dimensional gallium oxide monolayer for gas-sensing application," *The Journal of Physical Chemistry Letters*, vol. 12, no. 24, pp. 5813–5820, 2021.
- [8] P. Bergveld, J. Hendrikse, and W. Olthuis, "Theory and application of the material work function for chemical sensors based on the field effect principle," *Measurement science and technology*, vol. 9, no. 11, p. 1801, 1998.
- [9] A. A. Haque, S. G. Dhongade, and A. Singha, "Predictive analysis of gas sensing properties in a novel 2d gallium oxide phase," *IEEE Sensors Journal*, vol. 25, no. 8, pp. 12 644–12 652, 2025.
- [10] D. Raval, S. K. Gupta, and P. Gajjar, "Detection of h2s, hf and h2 pollutant gases on the surface of penta-pdas2 monolayer using dft approach," *Scientific Reports*, vol. 13, no. 1, p. 699, 2023.
- [11] S. Khammuang, A. Udomkijmongkol, S. Thasitha, T. Hussain, and K. Kotmool, "First-principles study insights into janus mowc-based mxenes for enhanced h2s and nh3 sensing applications," *Applied Surface Science*, vol. 699, p. 163110, 2025. [Online]. Available: <https://www.sciencedirect.com/science/article/pii/S0169433225008244>
- [12] S. Luo, R. Tu, W. Liu, J. Li, J. Li, K. Wang, J. Guo, S. Li, and X. Dai, "Adsorption of gas molecules (c2h6, co, h2s, ch2o, ch4, and co2) on gec monolayer: A first-principles study," *Computational and Theoretical Chemistry*, vol. 1249, p. 115263, 2025. [Online]. Available: <https://www.sciencedirect.com/science/article/pii/S2210271X25001999>
- [13] F. Opoku and P. P. Govender, "Two-dimensional cooh as a highly sensitive and selective h2s, hcn and hf gas sensor: A computational investigation," *Electroanalysis*, vol. 32, no. 12, pp. 2764–2774, 2020. [Online]. Available: <https://analyticalsciencejournals.onlinelibrary.wiley.com/doi/abs/10.1002/elan.202060337>
- [14] J. Zhu, Z. Xu, S. Ha, D. Li, K. Zhang, H. Zhang, and J. Feng, "Gallium oxide for gas sensor applications: A comprehensive review," *Materials*, vol. 15, no. 20, 2022. [Online]. Available: <https://www.mdpi.com/1996-1944/15/20/7339>
- [15] X. Zhang, L. Yu, X. Wu, and W. Hu, "Experimental sensing and density functional theory study of h2s and sof2 adsorption on au-modified graphene," *Advanced Science*, vol. 2, no. 11, p. 1500101, 2015. [Online]. Available: <https://advanced.onlinelibrary.wiley.com/doi/abs/10.1002/advs.201500101>
- [16] R. Majidi and A. Ramazani, "Detection of hf and h2s with pristine and ti-embedded twin graphene: A density functional theory study," *Journal of Physics and Chemistry of Solids*, vol. 132, pp. 31–37, 2019. [Online]. Available: <https://www.sciencedirect.com/science/article/pii/S0022369719302781>
- [17] N. Viveka, C. Poornimadevi, C. P. Kala, and D. J. Thiruvadigal, "Dft insights into the gas sensing properties of light platinum group metal (ru, rh & pd) doped mose2 monolayers," *Surfaces and Interfaces*, vol. 66, p. 106579, 2025. [Online]. Available: <https://www.sciencedirect.com/science/article/pii/S2468023025008363>
- [18] K. Xu, N. Liao, B. Zheng, and H. Zhou, "Adsorption and diffusion behaviors of h2, h2s, nh3, co and h2o gases molecules on moo3 monolayer: A dft study," *Physics Letters A*, vol. 384, no. 21, p. 126533, 2020. [Online]. Available: <https://www.sciencedirect.com/science/article/pii/S037596012030400X>
- [19] B. Liang, W. Li, Q. Ren, C. Zhu, and J. Li, "Gas adsorption performance of ta doped mose2 based on first principles," *Results in Physics*, vol. 42, p. 105978, 2022. [Online]. Available: <https://www.sciencedirect.com/science/article/pii/S2211379722005927>
- [20] Y. Yong, R. Gao, X. Wang, X. Yuan, S. Hu, Z. Zhao, X. Li, and Y. Kuang, "Highly sensitive and selective room-temperature gas sensors based on b6n6h6 monolayer for sensing so2 and nh3: A first-principles study," *Results in Physics*, vol. 33, p. 105208, 2022. [Online]. Available: <https://www.sciencedirect.com/science/article/pii/S2211379722000249>
- [21] S. F. Rastegar, A. A. Peyghan, and N. L. Hadipour, "Response of si- and al-doped graphenes toward hcn: A computational study," *Applied Surface Science*, vol. 265, pp. 412–417, 2013. [Online]. Available: <https://www.sciencedirect.com/science/article/pii/S0169433212019794>
- [22] J. Pang, Q. Yang, X. Ma, L. Wang, C. Tan, D. Xiong, H. Ye, and X. Chen, "Dft coupled with negf study of ultra-sensitive hcn and hnc gases detection and distinct i–v response based on phosphorene," *Phys. Chem. Chem. Phys.*, vol. 19, pp. 30 852–30 860, 2017. [Online]. Available: <http://dx.doi.org/10.1039/C7CP03941G>
- [23] C. Feng, H. Qin, D. Yang, and G. Zhang, "First-principles investigation of the adsorption behaviors of ch2o on bn, aln, gan, inn, bp, and p monolayers," *Materials*, vol. 12, no. 4, 2019. [Online]. Available: <https://www.mdpi.com/1996-1944/12/4/676>
- [24] S. Luo, R. Tu, W. Liu, J. Li, J. Li, K. Wang, J. Guo, S. Li, and X. Dai, "Adsorption of gas molecules (c2h6, co, h2s, ch2o, ch4, and co2) on gec monolayer: A first-principles study," *Computational and Theoretical Chemistry*, vol. 1249, p. 115263, 2025. [Online]. Available: <https://www.sciencedirect.com/science/article/pii/S2210271X25001999>
- [25] N. U. Rahman, A. A. Khan, R. Ullah, R. Ahmad, and I. Ahmad, "Selective sensing of nh3 and ch2o molecules by novel 2d porous hexagonal boron oxide (b3o3) monolayer: A dft approach," *Surfaces and Interfaces*, vol. 29, p. 101767, 2022. [Online]. Available: <https://www.sciencedirect.com/science/article/pii/S2468023022000487>
- [26] K. K. Ghuman, S. Yadav, and C. V. Singh, "Adsorption and dissociation of h2o on monolayered mos2 edges: Energetics and mechanism from ab initio simulations," *The Journal of Physical Chemistry C*, vol. 119, no. 12, pp. 6518–6529, 2015. [Online]. Available: <https://doi.org/10.1021/jp510899m>
- [27] Z. Cui, C. Xiao, Y. Lv, Q. Li, R. Sa, and Z. Ma, "Adsorption behavior of co, co2, h2, h2o, no, and o2 on pristine and defective 2d monolayer ferromagnetic fe3gete2," *Applied Surface Science*, vol. 527, p. 146894, 2020. [Online]. Available: <https://www.sciencedirect.com/science/article/pii/S0169433220316512>
- [28] J. Haruyama, T. Sugimoto, and O. Sugino, "First-principles study of water adsorption monolayer on pt(111): Adsorption energy and second-order nonlinear susceptibility," *Phys. Rev. Mater.*, vol. 7, p. 115803, Nov 2023. [Online]. Available: <https://link.aps.org/doi/10.1103/PhysRevMaterials.7.115803>
